# Supplementary material for: Domain Separation Networks
Source: arXiv:1608.06019 source file (2016-08-22)
Supplement: Supplementary file 1 [file appendix.tex]

Hyperparameters for CORAL:

Linear SVM for MNIST-M $\gamma=1e^{-4}$, SynNumbers: $\gamma = 1e^{-3}$, SVHN to MNIST: $\gamma = 1e^{-4}$,  GTSRB: $\gamma = 1e^{-4}$

ours

mnist_m lr_0.0132588_lambda_0.0110615_delta_0.392244 lr_0.0100109_lambda_0.0115405_delta_0.292813
svhn_to_mnist lr_0.010519_lambda_0.0168883_delta_0.195155
